# Supplementary material for: No Epoch Like the Present: Robust Climate Emulation Requires Out-of-Distribution Generalisation
Source: arXiv:2605.22248 source file (2026-05-21)
Supplement: Supplementary file 1 [file mlp_variants.tex]

\begin{table}[h]
\centering
\caption{Data, task, and hyperparameter search space for investigating if seasonal shift is a good proxy for climate change shift.}
\label{tab/mlp_variants}
\begin{tabular}{ll}
\hline
\textbf{Component} & \textbf{Specification} \\
\hline
Dataset & ERA5 monthly reanalysis~\cite{hersbach_era5_2020} \\
Resolution & 2.5$^\circ$ grid \\
Target & $\log(\mathrm{pr})$ (monthly precipitation) \\
Inputs & tas, zg500, prw \\
Prediction setup & Independent per grid point \\
Model class & Multi-layer perceptron (MLP) \\
Number of models & 200 \\
Depth & 2--6 layers \\
Width & 64--1024 hidden units \\
Dropout & 0--0.25 \\
Weight decay & $10^{-5}$--$10^{-2}$ \\
Learning rate & $5\times10^{-4}$--$10^{-2}$ \\
Search method & Random search \\
\hline
\end{tabular}
\end{table}
